# Supplementary material for: Minimising biases in Full Configuration Interaction Quantum Monte Carlo
Source: arXiv:1407.1753 ancillary file (2015-06-11)
Supplement: Supplementary file 1 [file supp_mat.pdf]

# Supplemental Material for "Unloading the dice: Minimising biases in Full Configuration Interaction Quantum Monte Carlo"

W. A. Vigor,[1] J. S. Spencer,[2,3] M. J. Bearpark,[1] and A. J. W. Thom[1,4]

[1] *Department of Chemistry, Imperial College London, Exhibition Road, London, SW7 2AZ, United Kingdom*

[2] *Department of Physics, Imperial College London, Exhibition Road, London, SW7 2AZ, United Kingdom*

[3] *Department of Materials, Imperial College London, Exhibition Road, London, SW7 2AZ, United Kingdom*

[4] *University Chemical Laboratory, Lensfield Road, Cambridge, CB2 1EW, United Kingdom*

(Dated: 11 June 2015)

## I. THE STATIONARY DISTRIBUTION OF $H_2$ IN A STO-3G BASIS SET

A simple choice of a two determinant system is singlet $H_2$ in a STO-3G basis. Here we present results to illustrate some of the properties of the transition matrix. All variables are as defined in the main text.

The population of psips in a simulation is controlled by two variables: $N_s$, the number of psips at which the shift is allowed to vary, and $\xi$, the shift damping. These degrees of freedom may be adjusted at the same time to achieve simulations with a given total number of psips but different population dynamics. The total population of psips should be stable when the shift is equal to the correlation energy if FCIQMC is not biased. Fig. 1 shows the shift as a function of population for pairs of $\xi$ and $N_s$ such that the average population is identical. $\xi$ and $N_s$ in turn affect the stationary distributions of the shift and the number of psips. If $\xi$ is large the stationary distribution of the number of psips is narrow because the population is well controlled, however the stationary distribution of the shift is broad (Fig. 2). Of course we can only choose $\xi$ and $N_s$ to achieve a desired population if we know the correlation energy. In practice one could use an estimate of the correlation energy from a less expensive method, such as coupled cluster theory, to reach an approximate desired population.

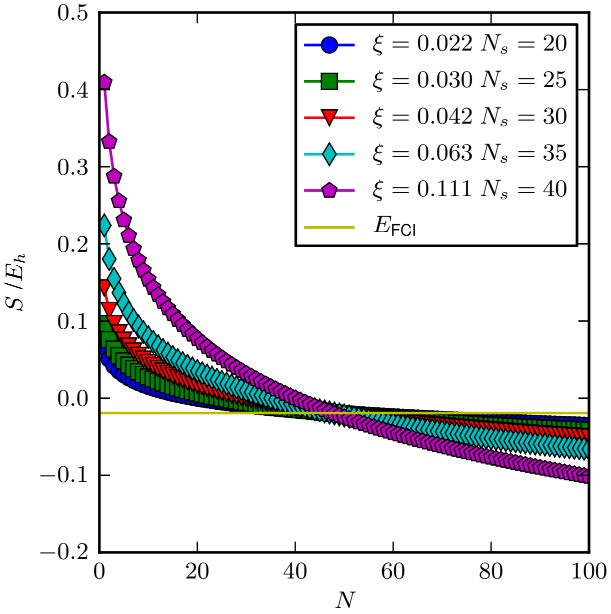


FIG. 1. The instantaneous shift, $S$, as a function of the instantaneous psip population, $N$, for $H_2$ (STO-3G basis, internuclear separation 0.7122Å[1]). The pairs of population control parameters, $\xi$ and $N_s$, were chosen such that $S$ equals the correlation energy at the same number of psips (47.63). Lines are drawn to guide the eye.

The shift parameters also affect the projected energy estimator. The population on each determinant is proportional to the overlap of that determinant with the ground state of the FCI wavefunction. Thus we expect the stationary distributions of both the denominator and numerator of the projected energy (Fig. 3) to look similar to the stationary distribution of the number of psips (Fig. 2), though the numerator is scaled by the appropriate Hamiltonian matrix element. Changing the $\xi$ and $N_s$ seem to have little effect on the numerator of the projected energy (Fig. 3) though the change in variance of the denominator indicates that the projected energy will have a smaller variance as $\xi$ increases.

Our tests indicate that the timestep has very little effect on the stationary distribution. This is not surprising as it simply scales all probabilities. We would expect the stationary distribution to change once the timestep is sufficiently large to cause multiple psips to be spawned or undergo death from a single psip.

[1]Hartree–Fock energy: $-1.1175058843\,E_h$.
[2]Hartree–Fock energy: $-0.9338980552\,E_h$.

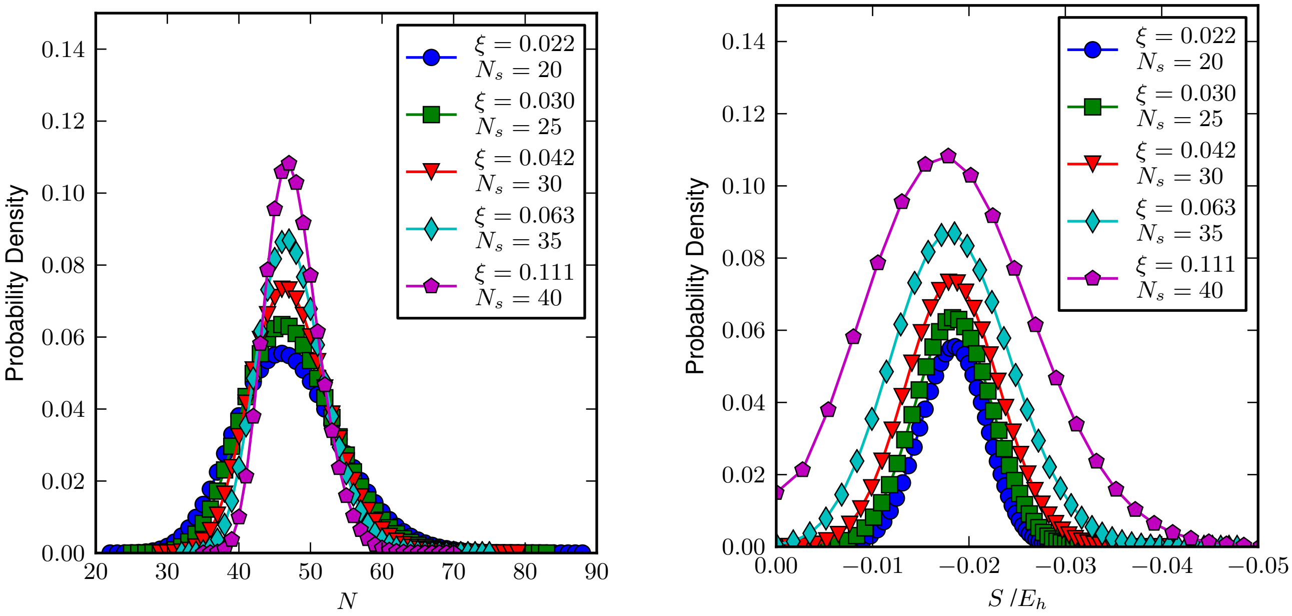


FIG. 2. The effect of population control on the stationary distributions of the number of psips, $N$, and the shift, $S$ for $H_2$ (STO-3G basis, internuclear separation 0.7122Å[1]). Only states with up to 100 psips on each determinant were included in the transition matrix. The variance of $N$ increases as $\xi$ decreases whereas the variance of $S$ increases as $\xi$ increases. Lines are drawn to guide the eye.

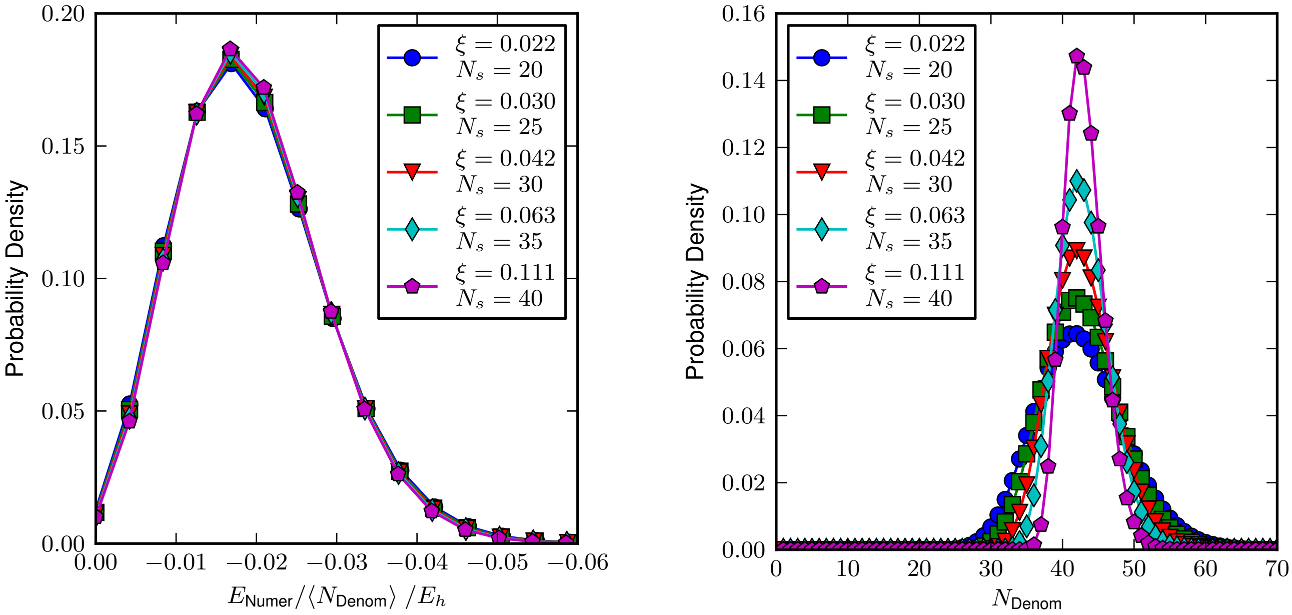


FIG. 3. The effect of population control on the stationary distribution on the numerator and denominator of the projected energy for $H_2$ (STO-3G basis, internuclear separation 1.4244Å[2]). Only states with up to 100 psips on each determinant were included in the transition matrix. The variance of the denominator increases as $\xi$ increases. Each numerator has been divided by the mean denominator for that set of parameters to place the plots on a common scale. The variance of the normalized numerator has only a small dependence on the population control parameter. Lines are drawn to guide the eye.
